# Supplementary material for: AppBench: Planning of Multiple APIs from Various APPs for Complex User Instruction
Source: arXiv:2410.19743 source file (2024-10-10)
Supplement: Supplementary file 1 [file data_analysis.tex]

\begin{table}[!t]
\setlength{\belowcaptionskip}{0pt}
    \centering
    \begin{adjustbox}{max width=1.0 \textwidth}
    \begin{tabular}{l | cccc}
    \toprule
    % dynamic / multi-turn?
    \textbf{Statistics} & \textbf{SS} & \textbf{SM} & \textbf{MS} & \textbf{MM} \\
    \hline
    \# Samples & 200 & 200 & 200 & 200 \\
    \# Apps & 9 & 11 & 10 & 11 \\
    \# APIs & 11 & 22 &12 & 23\\
    \hline
    Max Apps & 1 & 1 & 4 & 4\\
    Max APIs & 1 & 4 & 4 & 8\\
    Max. arguments & 6 & 7 & 6 & 7\\
    
    % Max. Para. & 1 &4 &4& 8 \\
    % Max. Seq.. & 1 &1 &4 & 3\\
    
    % Avg. Para. & 1 &2.2 &1.2& 1.9 \\
    % Avg. Seq. & 1 &1.0 &2.2 & 1.8\\
    
    % Avg. Apps & 1.0 & 1.0 & 2.7 & 2.2 \\
    % Avg. APIs & 1.0 & 2.2 & 2.7 & 3.3 \\
    % Avg. arguments & 4.0 & 4.5 & 3.8 & 4.4 \\
    \bottomrule
    \end{tabular}
    \end{adjustbox}
    \caption{The data statistics of our proposed \texttt{MetaBench}.}
    \label{tab:data_ana}
\end{table}
